# Supplementary material for: Linear Coding for AWGN channels with Noisy Output Feedback via Dynamic Programming
Source: arXiv:2103.10807 source file (2022-05-23)
Supplement: Supplementary file 1 [file 9Appendix.tex]

\section{Appendix}

\subsection{Proof of Remark~\ref{Remark: SK scheme as sequentially linear}}
\label{App: SK scheme as sequentially linear}

\begin{proof}
  \textit{\sk scheme as a sequential scheme}

  The sequence of receiver's \mmse estimates $\{\hat{w}_0,\hat{w}_1,\hat{w}_2,\cdots\}$ satisfies the following recursive equation
  \begin{align*}
    \hat{w}_t = \hat{w}_{t-1} + \E[u_t|y_t],
  \end{align*}
  where $u_t = w - \hat{w}_{t-1}$ denotes the error in the most recent estimate of $w$ and the estimation error $u_t$ and $y_t$ is the received signal observed as feedback at the encoder. This is derived from the fact that the error in estimate $u_t$ is orthogonal to all the observations till time $t$, $y^{0:t-1}$. Therefore, the encoding process is sequential, $u_{t+1} = u_{t} - \E[u_{t}|y_{t}]$. The transmitted symbol $x_{t+1}$ is a scaled version of $u_t$.
  \begin{align*}
    u_{t+1} & = w - \hat{w}_{t}                                           \\
            & = \cq{w - \hat{w}_{t-1}} - \cq{\hat{w}_{t} - \hat{w}_{t-1}} \\
            & = u_{t} - \E\sq{u_{t}|y_{t}},
  \end{align*}
  The transmitter sends $x_t = \gamma_t u_t$, where $\gamma_t$ denotes the power normalization constant. Under the average peak power assumption, $\gamma_t = \sqrt{P/\E[u_t^2]}$.
  The estimation error can be also represented in a recursive equation; after $t$ transmissions, the error in the estimate of $w$ reduces is $\E[(w-\hat{w})^2] =  \sigma_w^2/{\cq{1+P}^T}$, which decays exponentially in $P$ (See~\cite{Gallager2010} for a detailed derivation).  This scheme is analytically shown to be {\em optimal} for communication of Gaussian messages~\cite{}.
\end{proof}

\subsection{Proof of Remark~\ref{Remark: chance and love as sequentially linear}}
\label{App: chance and love as sequentially linear}

\begin{proof}
  The authors in~\cite{Chance2011a} propose a scheme for channels with noisy feedback as
  \begin{align}
    x_{t+1} = \bld{F}_t\bld{\zt} +\bld{g} w, \label{Eqn: chance and love transmission equation}
  \end{align}
  where $x_{t+1}$ is the transmitted symbol, $\bld{\zt}_t$ is the noise vector, $\bld{n}_t +\bld{\nt}_t$, and $w$ is the intended message. The scheme is parameterized through the encoding matrix $\bld{F}$ which is a lower triangular Toeplitz matrix given as
  \begin{align*}
    \bm{0                                          &         & \cdots                            &                                               & 0 \\
    -\frac{1-\beta_0^2}{\cq{1-\sigma_b^2}\beta_0}  & 0       &                                   &                                               & . \\
    -\frac{1-\beta_0^2}{1+\sigma_b^2}              & \ddots  & \ddots                            & .                                             & . \\
    \vdots                                         &         &                                   &                                               &   \\
    -\frac{1-\beta_0^2}{1+\sigma_b^2}\beta_0^{T-3} & .\cdots & -\frac{1-\beta_0^2}{1+\sigma_b^2} & -\frac{1-\beta_0^2}{\cq{1-\sigma_b^2}\beta_0} & 0 \\
    }
  \end{align*}
  while $\bld{g}$ is given as
  \begin{align*}
    \bld = \sqrt{\frac{1-\beta_0^2}{1-\beta_0^{2\cq{T+1}}}}\bm{1 & \beta_0 & \beta_0^2 & \cdots & \beta_0^{T}}^T
  \end{align*}
  The value of $\beta_0$ is obtained as a solution to the equation (31) of the paper. Here, we show that the scheme is sequential and linaer in terms of the feedback and the past symbols.

  From~\eqref{Eqn: chance and love transmission equation}, we can represent the transmitted symbol at any instant $t$ as
  \begin{align*}
    x_{t+1} & = \sqrt{\frac{1-\beta_0^2}{1-\beta_0^{2\cq{T+1}}}} \beta_0^{t+1} w + \bm{-\frac{1-\beta_0^2}{1+\sigma_b^2}\beta_0^{t}            & -\frac{1-\beta_0^2}{1+\sigma_b^2}\beta_0^{t-1} & \cdots -\frac{1-\beta_0^2}{\cq{1-\sigma_b^2}\beta_0}} \bld{\zt}^{t}                                                     \\
            & = \sqrt{\frac{1-\beta_0^2}{1-\beta_0^{2\cq{T+1}}}} \beta_0^{t+1} w + \bm{-\frac{1-\beta_0^2}{1+\sigma_b^2}\beta_0^{t}            & -\frac{1-\beta_0^2}{1+\sigma_b^2}\beta_0^{t-1} & \cdots -\frac{1-\beta_0^2}{\cq{1-\sigma_b^2}}} \bld{\zt}^{t-1} +  -\frac{1-\beta_0^2}{\cq{1-\sigma_b^2}\beta_0}\zt_{t}  \\
            & = \beta_0\cq{\sqrt{\frac{1-\beta_0^2}{1-\beta_0^{2\cq{T+1}}}} \beta_0^{t} w + \bm{-\frac{1-\beta_0^2}{1+\sigma_b^2}\beta_0^{t-1} & -\frac{1-\beta_0^2}{1+\sigma_b^2}\beta_0^{t-2} & \cdots -\frac{1-\beta_0^2}{\cq{1-\sigma_b^2}}} \bld{\zt}^{t-1}} +  -\frac{1-\beta_0^2}{\cq{1-\sigma_b^2}\beta_0}\zt_{t} \\
            & = \beta_0 x_t +  -\frac{1-\beta_0^2}{\cq{1-\sigma_b^2}\beta_0}\cq{\yt_t - x_t}                                                                                                                                                                                                                              \\
            & = \cq{\beta_0 + -\frac{1-\beta_0^2}{\cq{1-\sigma_b^2}\beta_0}}x_t +  -\frac{1-\beta_0^2}{\cq{1-\sigma_b^2}\beta_0}\yt_t                                                                                                                                                                                     \\
  \end{align*}
  We represent the current transmitted symbol $x_{t+1}$ in terms of the past symbol $x_t$ and the received feedback $\yt_t$. This establishes the sequential nature of the scheme.

\end{proof}

\subsection{Proof of Remark~\ref{Remark: cl and our scheme are analogous}}
\label{App: cl and our scheme are analogous}

\begin{proof}
  The scheme derived from our proposed dynamic program shares the same pattern, and thus all the results that hold for the scheme proposed by Chance and Love also hold for our scheme. Additionally, our scheme is obtained without any conjectures on the scheme's structure.

  Any $t^{th}$ transmission can be expressed in terms of the matrices $\boldsymbol{F}$ and $\bld{g}$ as
  \begin{align*}
    x_{t+1} = \bld{F}\sq{t:}\zt^{1:t} + \bld{g}w
  \end{align*}
  where $\zt = \nt + n_t$ is the sum of the forward and the feedback noise realizations.
  where $\bld{F}$ represents the $t^{th}$ row of the matrix. From the matrix operation, we can deduce that the same equation can be expressed in terms of the past transmitted symbol and the new feedback as
  \begin{align}
    x_{t+1} = \beta_0 x_t + \frac{1-\beta_0^2}{\cq{1- \sigma_b^2}\beta_0}y_t + w
  \end{align}
  This is establishes the sequential nature of the encoding scheme proposed by Chance and Love in their paper and the same being an outcome of our scheme.

  \begin{align*}
    \bm{0                                            &                                                  & \cdots &                                           & 0               \\
    \gamma_1c_0                                      & 0                                                &        &                                           & .               \\
    \gamma_2\cq{1+\gamma_1c_1}c_0                    & \gamma_2c_1                                      & \ddots & .                                         & .               \\
    \vdots                                           &                                                  &        &                                           &                 \\
    \gamma_T\prod_{t = 1}^{T-1}\cq{1+\gamma_tc_t}c_0 & \gamma_T\prod_{t = 2}^{T-1}\cq{1+\gamma_tc_t}c_1 & \cdots & \gamma_T\cq{1+\gamma_{T-1}c_{T-1}}c_{T-2} & \gamma_Tc_{T-1} \\
    }
  \end{align*}

\end{proof}

\subsection{Proof of Theorem~\ref{Thm: Solution of the dynamic program}}
\label{App: Solution of the dynamic program}

\begin{proof}[Proof of Theorem~\ref{Thm: Solution of the dynamic program}]

  At time $t=T-1$, from~\eqref{Eqn: Optimal Policy Derivation}, we find $\at_{T-1}$ through $\frac{\partial V_T}{\partial a_{T-1}}=0$ which leads to
  \begin{align*}
    \tilde{a}_{T-1} = - \frac{\sqrt{S}\cq{\frac{\sigma_{u,T-1}}{\sigma_f}}}{\eta_0},
  \end{align*}
  where all the symbols have been defined in Theorem~\ref{Thm: Solution of the dynamic program}. Therefore, the optimal transmission scheme is given as,
  \begin{align*}
    \tilde{\phi}_{T-1}\cq{u_{T-1},\yt_{T-1}} = \sqrt{\frac{P}{\sigma_{u,T}^2}}\cq{u_{T-1} - \frac{\sqrt{S}\cq{\frac{\sigma_{u,T-1}}{\sigma_f}}}{\eta_0}\yt_{T-1}}.
  \end{align*}
  The value function that captures the \mse if we use the optimal policy from $t=T-1$ till $T$ which is given as
  \begin{align*}
    V_{T-1}\cq{s_{T-1}} = \frac{-\cq{\epsilon_{uw, {T-1}}}^4 + K_1\cq{\epsilon_{w, T-1}\sigma_{u, {T-1}}}^2 + \cq{\epsilon_{w, T-1}\epsilon_{u, T-1}}^2}{K_1\sigma_{u, T-1}^2+\cq{\epsilon_{u,T-1}}^2}
  \end{align*}
  where
  \begin{align*}
    K_1  = \frac{1+\beta +S\beta}{\cq{1+\beta}S\cq{1+S}}  = \frac{\eta_1}{\eta_3}
  \end{align*}
  We repeat the same procedure for $t = T-2$, $t = T-3$ and for any general $t$ and obtain corresponding $\tilde{\phi}$ and $V$ as
  \begin{align*}
    \tilde{\phi}_{T-2} & = \frac{\sqrt{P}}{\sigma_{u,T-1}}\cq{u_{T-2} - \frac{K_{2}\sqrt{S}\cq{\frac{\sigma_{u,T-2}}{\sigma_f}}}{K_{2}\eta_0 + \beta}\yt_{T-2}}                                          \\
    V_{T-2}            & = \frac{-\cq{\epsilon_{uw, T-2}}^4 + K_{2}\cq{\epsilon_{w, T-2}\sigma_{u, T-2}}^2 + \cq{\epsilon_{w, T-2}\epsilon_{u, T-2}}^2}{K_{2}\sigma_{u, T-2}^2+\cq{\epsilon_{u,T-2}}^2}, \\
    \tilde{\phi}_{T-3} & = \frac{\sqrt{P}}{\sigma_{u,T-2}}\cq{u_{T-3} - \frac{K_{3}\sqrt{S}\cq{\frac{\sigma_{u,T-3}}{\sigma_f}}}{K_{3}\eta_0 + \beta}\yt_{T-3}}                                          \\
    V_{T-3}            & = \frac{-\cq{\epsilon_{uw, T-3}}^4 + K_{3}\cq{\epsilon_{w, T-3}\sigma_{u, T-3}}^2 + \cq{\epsilon_{w, T-3}\epsilon_{u, T-3}}^2}{K_{3}\sigma_{u, T-3}^2+\cq{\epsilon_{u,T-3}}^2}, \\
    \tilde{\phi}_t     & = \frac{\sqrt{P}}{\sigma_{u,t+1}}\cq{u_{t} - \frac{K_{T-t}\sqrt{S}\cq{\frac{\sigma_{u,t}}{\sigma_f}}}{K_{T-t}\eta_0 + \beta}\yt_{t}}                                            \\
    V_{t}              & = \frac{-\cq{\epsilon_{uw, t}}^4 + K_{T-t}\cq{\epsilon_{w, t}\sigma_{u, t}}^2 + \cq{\epsilon_{w, t}\epsilon_{u, t}}^2}{K_{T-t}\sigma_{u, t}^2+\cq{\epsilon_{u,t}}^2},
  \end{align*}
  where
  \begin{align*}
    K_{2} & = \frac{\eta_1 K_{1}^2 + \eta_2K_{1}}{\eta_3K_{1}^2 + \eta_4K_{1}+\eta_2} = f\cq{K_{1}}.                           \\
    K_{3} & = \frac{\eta_1 K_{2}^2 + \eta_2K_{2}}{\eta_3K_{2}^2 + \eta_4K_{2}+\eta_2} = f\cq{K_{2}}.                           \\
    K_{t} & = \frac{\eta_1 K_{t-1}^2 + \eta_2K_{t-1}}{\eta_3K_{t-1}^2 + \eta_4K_{t-1}+\eta_2} = f\cq{K_{t-1}}=f^{t-1}\cq{K_1}.
  \end{align*}

  \textbf{Significance of $\mathbf{K_n}$:}
  We observe that the structure of the value expression $V_t$ with respect to the state $s_t$ remain similar barring the value of $K$ which is a function of system parameters $P$, $\sigma_f^2$ and $\sigma_b^2$ and $T$. Therefore, the value function $V_t$ and the optimal policy at any instant $t$ can be obtained by computing $K_1$ given in~\eqref{Eqn: K1 Value} and then applying the function $f\cq{\cdot}$ in~\eqref{Eqn: Kn Recursion}, $T-t-1$ times to obtain $K_{T-t}$. This formulation helps us in determining the value function (=\mse) and the optimal policy for any number of iterations and for any value of feedback variance without worrying about the increase in complexity.

\end{proof}

\subsection{Proof to Theorem~\ref{Thm: MSE Expression}}
\label{App: MSE Expression}

\begin{proof}
  Value function $V_t\cq{s_t}$ at any instant represents the error variance if we start from the state $s_t=\bq{\Sigma_t,\sigma_{u,t}^2}$, and use the optimal transmission scheme till time terminal transmission $T$. In other words,
  \begin{align}
    \text{MSE} = V_0\cq{S_0}
  \end{align}
  where $S_0$ is the state of the system in terms of the encoder and the decoder variances. More specifically, the value function $V_0\cq{S_0}$ gives the value of $\epsilon_{w,T}^2$ that we end up with after $n = T$ transmissions if we follow the optimal encoding policy $\phi_{0:T-1}$ from first transmission. This is specified as

  \begin{align}
    \text{MSE} & = V_0\cq{S_0}                                                                                                                                                                        \\
               & = \frac{-\epsilon_{uw, 0}^4 + K_T\cq{\epsilon_{w, 0}\sigma_{u, 0}}^2 + \cq{\epsilon_{w, 0}\epsilon_{u, 0}}^2}{K_T\sigma_{u, 0}^2+\cq{\epsilon_{u,0}}^2}, \label{Eqn:value_func_at_0}
  \end{align}
  where $S_0 = \bq{\Sigma_0, \sigma_{u,0}^2}$. Now, let us find the values for each constituent of $S_0$ after the raw transmission.

  Given the initial transmission of the original message $w$:
  \begin{align*}
    y_0            & =\gamma_0w + n_0^f                                            \\
    \sigma_{u,0}^2 & = \sigma_w^2                                                  \\
    \Sigma_0       & = \bm{\frac{\sigma_w^2}{S + 1} & \frac{\sigma_w^2}{S + 1} & 0 \\ \frac{\sigma_w^2}{S + 1} & \frac{\sigma_w^2}{S + 1} &0\\ 0&0&0}
  \end{align*}

  We substitute these values in $V_0$ of [relevant equations] to get
  \begin{align}
    V_0\cq{\Sigma_0^s,\Sigma_0^r} = \frac{\sigma_w^2}{\zeta_T} \label{Eqn:actual_mse_val}
  \end{align}
  where
  \begin{align}
    \zeta_T & = \frac{\cq{1+K_T+SK_T}\cq{K_T + \beta + \beta K_T + SK_T + 2S\beta K_T}}{\cq{K_T}\cq{K_T + \beta + \beta K_T + S\beta K_T}} \\
            & = \cq{1 + S + \frac{1}{K_T}}\cq{\frac{\frac{\eta_2}{K_T} + \eta_4}{\frac{\eta_2}{K_T} + \eta_1}} \label{Eqn:zeta_actual1}
  \end{align}
  We obtain the value of $K_T$ from~\eqref{Eqn: Kn Value},~\eqref{Eqn: Kn Recursion} and~\eqref{Eqn: K1 Value} as
  \begin{align}
    K_T = f^{T-1}\cq{K_1}
  \end{align}
  The values are obtained by computing $K_1=\frac{\eta_1}{\eta_3}$ and then recursively using the function $f$ $T$ times on it.

  The \mse for our algorithm after end of $T$ re-transmissions was obtained in~\eqref{Eqn:actual_mse_val}.
\end{proof}

\begin{proof}
  We begin with the derivation of the close form expression for \mse followed by appropriate assumptions to derive the asymptotic expression to prove the dependence on $T$ in a polynomial fashion. We analyze the asymptotic behavior of the expression. We show that the term $\text{\mse}$ derived in [relevent equations] is exponential in $T$ for noiseless case and is polynomial in $T$ for the noisy case in the following theorem.

  We have already established earlier that the value function expressions for any state $\cq{\Sigma_t, \sigma_{u,t}^2}$ depend on the parameter function $K_t$ which is computed by applying the function $f$ recursively starting from $K_1$ through the number of remaining transmissions $t-T$.

  The value $K$ in turn is defined through the system parameters of power constraint $P$, the forward noise variance $\sigma^2_f$, and the feedback noise variance $\sigma_b^2$. In order to study the growth of $V_0$ with respect to $T$ we study the behavior of $K_1$ through $K_T$.

  We begin by studying the series $K_n$, $n = 1\ldots t$ progressively based on the function $f$. We establish that $K_n$ is a harmonic series for the noisy feedback case where $\sigma_b\neq 0$ and is a geometric series for the noiseless case where $\sigma_b=0$ and for large $n$, where
  \begin{align}
    K_n = \frac{\eta_1 K_{n-1}^2 + \eta_2K_{n-1}}{\eta_3K_{n-1}^2 + \eta_4K_{n-1}+\eta_2}.
  \end{align}
  as defined in~\eqref{Eqn: Kn Value}.

  \blue{Transfer these equations to the appendix}
  \textbf{Case Noiseless Feedback:} $\sigma_b$ = 0

  \begin{align}
    \text{or}\quad \frac{1}{K_T} & = \cq{1+S}^T\frac{1}{K_1}                                     \\
                                 & = \cq{1+S}^T\frac{\eta_3}{\eta_4} \label{Eqn: noiseless 1/KT}
  \end{align}

\end{proof}

\begin{proof}
  We begin with the derivation of the close form expression for \mse followed by appropriate assumptions to derive the asymptotic expression to prove the dependence on $T$ in a polynomial fashion. We analyze the asymptotic behavior of the expression. We show that the term $\text{MSE}$ derived in [relevent equations] is exponential in $T$ for noiseless case and is polynomial in $T$ for the noisy case in the following theorem.

  We have already established earlier that the value function expressions for any state $\cq{\Sigma_t, \sigma_{u,t}^2}$ depend on the parameter function $K_t$ which is computed by applying the function $f$ recursively starting from $K_1$ through the number of remaining transmissions $t-T$.

  The value $K$ in turn is defined through the system parameters of power constraint $P$, the forward noise variance $\sigma^2_f$, and the feedback noise variance $\sigma_b^2$. In order to study the growth of $V_0$ with respect to $T$ we study the behavior of $K_1$ through $K_T$.

  We begin by studying the series $K_n$, $n = 1\ldots t$ progressively based on the function $f$. We establish that $K_n$ is a harmonic series for the noisy feedback case where $\sigma_b\neq 0$ and is a geometric series for the noiseless case where $\sigma_b=0$ and for large $n$, where
  \begin{align}
    K_n = \frac{\eta_1 K_{n-1}^2 + \eta_2K_{n-1}}{\eta_3K_{n-1}^2 + \eta_4K_{n-1}+\eta_2}.
  \end{align}

  as defined in~\eqref{}.

  \blue{Transfer these equations to the appendix}

  \textbf{Case Noisy Feedback:}

  Here we show that the common difference between the reciprocal terms of $K_n$ are constant.

  \begin{align}
    \frac{1}{K_n} - \frac{1}{K_{n-1}} = \frac{\eta_3K_{n-1} + \eta_4-\eta_1}{\eta_1K_{n-1} + \eta_2} \label{Eqn:common_diff_actual}
  \end{align}
  Assuming that $K_n$ becomes much smaller with increasing $n$ we get,
  \begin{align}
    \frac{1}{K_n} - \frac{1}{K_{n-1}} = \frac{\eta_4-\eta_1}{\eta_2} \\
    \text{i.e.}\quad \frac{1}{K_T} = \frac{1}{K_1} + \frac{\eta_4-\eta_1}{\eta_2}T \label{Eqn:KT_approx_expr}
  \end{align}
  This approximation holds true for any value of $T$ and with high value of $T$ the difference between the exact and the approximate expression goes down to zero.

  Now, the \mse expression at any instant $t$ and $n=T-t$ given in~\eqref{Eqn:value_func} can be approximate by using the harmonic progression series for $K_n$ which was shown in Lemma~\ref{Lemma:K_n-series}. Thus we can obtain a very close approximation for the error variance after $T$ transmissions without the need to solve the \dpp or having to use the function $f$ recursively, through a single expression given by.
  \begin{align}
    \text{\mse} = \frac{\sigma_w^2}{\zeta_T}
  \end{align}

  where
  \begin{align}
    \zeta_T & = \frac{\cq{\cq{\eta_1\eta_4 - \eta_1^2}T + \eta_2\eta_3 + \eta_1\eta_4}{\cq{\cq{\eta_1\eta_4 - \eta_1^2}T + \eta_2\eta_3 + \eta_1\eta_2\cq{S+1}}}}{\eta_1\eta_2\cq{\cq{\eta_1\eta_4 - \eta_1^2}T + \eta_2\eta_3 + \eta_1^2}}                                \\
            & = \frac{\cq{\frac{\eta_4 - \eta_1}{\eta_2}T + \frac{\eta_2\eta_3 + \eta_1\eta_4}{\eta_1\eta_2}}\cq{\frac{\eta_4 - \eta_1}{\eta_2}T + \frac{\eta_2\eta_3}{\eta_1\eta_2}+S+1}}{\frac{\eta_4 - \eta_1}{\eta_2}T + \frac{\eta_2\eta_3 + \eta_1^2}{\eta_1\eta_2}}
  \end{align}
  This expression can be obtained by substituting for $K_T$ in~\eqref{Eqn:zeta_actual1} with the expression obtained in~\eqref{Eqn:KT_approx_expr}.

  {\color{blue} Why we introduce this approximation: Chance-Love approx} The approximate value for \mse for high value of $T$ can be expressed as
  \begin{align}
    \text{MSE} \approx \frac{\sigma_w^2}{\zeta^\star}, \text{\ where\ } \label{Eqn:MSE_approx}
  \end{align}
  \begin{align}
    \zeta^\star & = \cq{\frac{\eta_4 - \eta_1}{\eta_2}}T                     \\
                & = \cq{\frac{S +S\beta}{\beta}}T = S\cq{1+\frac{1}{\beta}}T
  \end{align}

  This is same as the asymptotic bound that was found in~\cite{Cover2003} and in~\cite{Chance2011a}.
\end{proof}
